# Supplementary material for: Jointly Detecting and Separating Singing Voice: A Multi-Task Approach
Source: arXiv:1804.01650 ancillary file (2018-04-05)
Supplement: Supplementary file 1 [file max_likelihood_appendix.pdf]

# Jointly Detecting and Separating Singing Voice: A Multi-Task Approach Appendix

This appendix will theoretically derive a probabilistically grounded loss function for the problem of joint singing voice detection and separation.

Let  $m$  be the input spectrogram to the model represented as a vector of dimensionality  $T \cdot F$ , where  $T$  is the number of time frames, and  $F$  is the number of frequency bins in the spectrogram. Let  $s$  describe the combination of an accompaniment and voice source spectrogram excerpt with a vector of dimensionality  $d = 2 \cdot T \cdot F$ . Furthermore, let  $o \in \{0, 1\}^T$  be a binary vector of dimensionality  $T$  describing vocal activity labels at each time frame of an audio excerpt  $m$ .

We define a model with parameters  $\phi$  that yields the probability distribution  $p_\phi(s, o|m)$  mapping mixtures to accompaniment and vocal tracks and predict vocal activity. Following the Multi-Task learning principle, the model internally calculates a hidden representation so that the outputs become independent of each other under this hidden representation:  $p_\phi(s, o|m) = p_\phi(s|h) \cdot p_\phi(o|h) \cdot p_\phi(h|m)$ . We will focus on a deterministic prediction of  $h$  using a function  $f_\phi^h : m \rightarrow h$ .

We now consider the overall joint probability  $p_\phi(m, h, s, o)$ , viewing our model as a data generator that we can train according to Maximum Likelihood. Since we always condition on the mixture input  $m$ , we set  $p(m)$  to the true distribution of mixtures so that our model always predicts based on real mixture inputs which are not modeled itself. Therefore, we can decompose the joint probability as  $p_\phi(m, h, s, o) = p_D(m) \cdot p_\phi(s, o|m)$ , where  $p_D$  is the empirical data distribution, and our parameters only model the conditional likelihood.

Now assume we have a multi-track dataset and mixtures with vocal activity labels available with  $N$  and  $M$  observations, respectively. Applying the principle of Maximum likelihood for a generative model with missing data, we can define the following log-likelihood function:

$$L_\phi = \sum_{i=1}^N \log p_\phi(s_i, m_i) + \sum_{j=1}^M \log p_\phi(o_j, m_j) \quad (1)$$

We compute the above marginal probabilities by marginalising out the respectively missing variables. For the first term, this means

$$\begin{aligned}
\log p_\phi(s, m) &= \log \int_h \sum_o p(m) p_\phi(s, o|m) dh \\
&= \log p_D(m) + \log \int_h \sum_o [p_\phi(s|h) \cdot p_\phi(o|h) \cdot p_\phi(h|m)] dh \\
&\propto_\phi \log \int_h [p_\phi(s|h) p_\phi(h|m)] dh \\
&\approx \log p_\phi(s | f_\phi^h(m)) \\
&:= \log \mathcal{N}(s | f_\phi^s(f_\phi^h(m_i)), \sigma^2 \mathbf{I}_d)
\end{aligned} \tag{2}$$

Integration and summation over  $h$  and  $o$  respectively occurs over all its dimensions. Note that the dependency on  $o$  disappears, since we integrate  $p(o|h)$  over all  $o$ . In the second last line, the sampling over  $h$  is replaced by the output of the deterministic function  $f_\phi^h$ . In the last line, we further define the output likelihood over the joint sources as a normal distribution with a mean given as output of our model, and a learnable scalar  $\sigma^2$  as isotropic variance in each dimension.  $\mathbf{I}_d$  denotes the  $d \times d$  identity matrix.

For the likelihood of mixtures with vocal activity labels  $p_\phi(o, m)$ , we can make similar simplifications. Firstly, we set the probability of a vocal activity curve to be equal to the product of probabilities at each time step  $t$ :

$$\begin{aligned}
p_\phi(o, m) &= \prod_{t=1}^T p_\phi(o^t, m) \\
\Rightarrow \log p_\phi(o, m) &= \sum_{t=1}^T \log p_\phi(o^t, m)
\end{aligned} \tag{3}$$

Then, we compute  $\log p_\phi(o^t, m)$  as follows:

$$\begin{aligned}
\log p_\phi(o^t, m) &\propto_\phi \log \int_h [p_\phi(o^t|h) p_\phi(h|m)] dh \\
&\approx \log p_\phi(o^t | f_\phi^h(m)) \\
&= o^t \cdot \log \sigma(f_\phi^o(f_\phi^h(m))) + (1 - o^t) \cdot \log(1 - \sigma(f_\phi^o(f_\phi^h(m)))) \\
&= -H(o^t, \sigma(f_\phi^o(f_\phi^h(m))))
\end{aligned} \tag{4}$$

The binary cross-entropy is denoted by  $H$ . We see that when defining  $p_\phi(o^t|m)$  to be  $\sigma(f_\phi^o(f_\phi^h(m)))$  with  $\sigma$  as sigmoid function, we arrive at minimising the binary cross-entropy between label  $o^t$  and prediction at each time step  $t$ .

We combine the above terms for separation predictions with a Normal likelihood from (??) and the binary cross-entropy terms from (??) to determine the log-likelihood from (??) on the combined data:

$$\begin{aligned}
L_\phi &= \sum_{i=1}^N \log p_\phi(s_i, m_i) + \sum_{j=1}^M \sum_{t=1}^T \log p_\phi(o_j, m_j) \\
&\propto_\phi \sum_{i=1}^N \log \mathcal{N}(s | f_\phi^s(f_\phi^h(m_i)), \sigma^2 \mathbf{I}_d) - \sum_{j=1}^M \sum_{t=1}^T H(o_j^t, \sigma(f_\phi^o(f_\phi^h(m_j)))) \\
&\propto_\phi \sum_{i=1}^N \left( -\frac{1}{2\sigma^2} \|s_i - f_\phi^s(m_i)\|^2 - d \log \sigma \right) - \sum_{j=1}^M \sum_{t=1}^T H(o_j^t, \sigma(f_\phi^o(f_\phi^h(m_j)))) \\
&= -\frac{1}{2\sigma^2} \sum_{i=1}^N \|s_i - f_\phi^s(m_i)\|^2 - Nd \log \sigma - \sum_{j=1}^M \sum_{t=1}^T H(o_j^t, \sigma(f_\phi^o(f_\phi^h(m_j))))
\end{aligned} \tag{5}$$

Note that we include  $\sigma^2$  as a learnable parameter so we cannot further simplify from here.

One issue with directly using this loss function for training is the scaling. With more data points (larger  $N$  and  $M$ ), or with a larger dimensionality  $d$  of the source output space, the loss varies more, since we have more summands in the former case and more summation over quadratic differences in the latter case. When using the loss for stochastic gradient descent, this means that the size of gradients varies strongly depending on the usage scenario, which can impede learning. To make the loss independent of dataset size and dimensionality of the source output, we divide by  $N + M$  and  $d$ :

$$\begin{aligned}
\hat{L}_\phi &:= \frac{L_\phi}{(N+M)d} = \\
&- \frac{1}{2\sigma^2(N+M)} \sum_{i=1}^N \text{MSE}(s_i, f_\phi^s(f_\phi^h(m_i))) \\
&- \frac{N}{N+M} \log \sigma \\
&- \frac{1}{2F} \frac{1}{N+M} \sum_{j=1}^M \frac{1}{T} \sum_{t=1}^T H(o_j^t, \sigma(f_\phi^o(f_\phi^h(m_j))))
\end{aligned} \tag{6}$$

MSE defines the mean squared error between source ground truth and prediction. Due to division by  $d = 2TF$ , the cross-entropy term for each sample  $m_i$  can now be seen as the average over the cross-entropy terms for each vocal activity label  $o^t$ .

We can write the naive loss combining MSE and average cross-entropy, as used in the main paper, as

$$I = \alpha \frac{1}{N} \sum_{i=1}^N \text{MSE}(s_i, f_\phi^s(f_\phi^h(m_i))) + (1-\alpha) \frac{1}{M} \sum_{j=1}^M \frac{1}{T} \sum_{t=1}^T H(o_j^t, \sigma(f_\phi^o(f_\phi^h(m_j)))) \tag{7}$$

We observe that maximising our scaled log-likelihood from (??) is equivalent to minimising the naive loss, when fixing the variance parameter  $\sigma^2$  and the weighting  $\alpha$  to a specific value:

$$\begin{aligned}
\hat{L}_\phi &= -I - \frac{N}{N+M} \log \sigma \text{ if} \\
\alpha &= \frac{1}{2\sigma^2} \frac{N}{N+M} \text{ and} \\
1-\alpha &= \frac{1}{2F} \frac{M}{N+M} \text{ so that} \\
\sigma^2 &= \frac{FN}{2FN + 2MF - M}
\end{aligned} \tag{8}$$

Although our log-likelihood function is theoretically more satisfying as it avoids a hyper-parameter and naturally accounts for a different amount of samples in both datasets, empirically we did not achieve better performance using this loss. A reason might be the learning dynamics of an ADAM optimiser on a neural network combined with the loss scaling: As the learnable variance  $\sigma$  decreases during training, the loss grows in size and variance far beyond that of the naive loss, which might mean lower learning rates are needed. This should be investigated further.
